# Supplementary material for: Crypt$\epsilon$: Crypto-Assisted Differential Privacy on Untrusted Servers
Source: arXiv:1902.07756 source file (2020-03-10)
Supplement: Supplementary file 1 [file Graphs_Appendix.tex]

\begin{figure*}[ht]

    \begin{subfigure}[b]{0.25\linewidth}
        \centering
         \includegraphics[width=1\linewidth]{8_final.pdf}
        \caption{ Program 1}
        \label{fig:P1}
    \end{subfigure}%%
    \begin{subfigure}[b]{0.25\linewidth}
    \centering \includegraphics[width=1\linewidth]{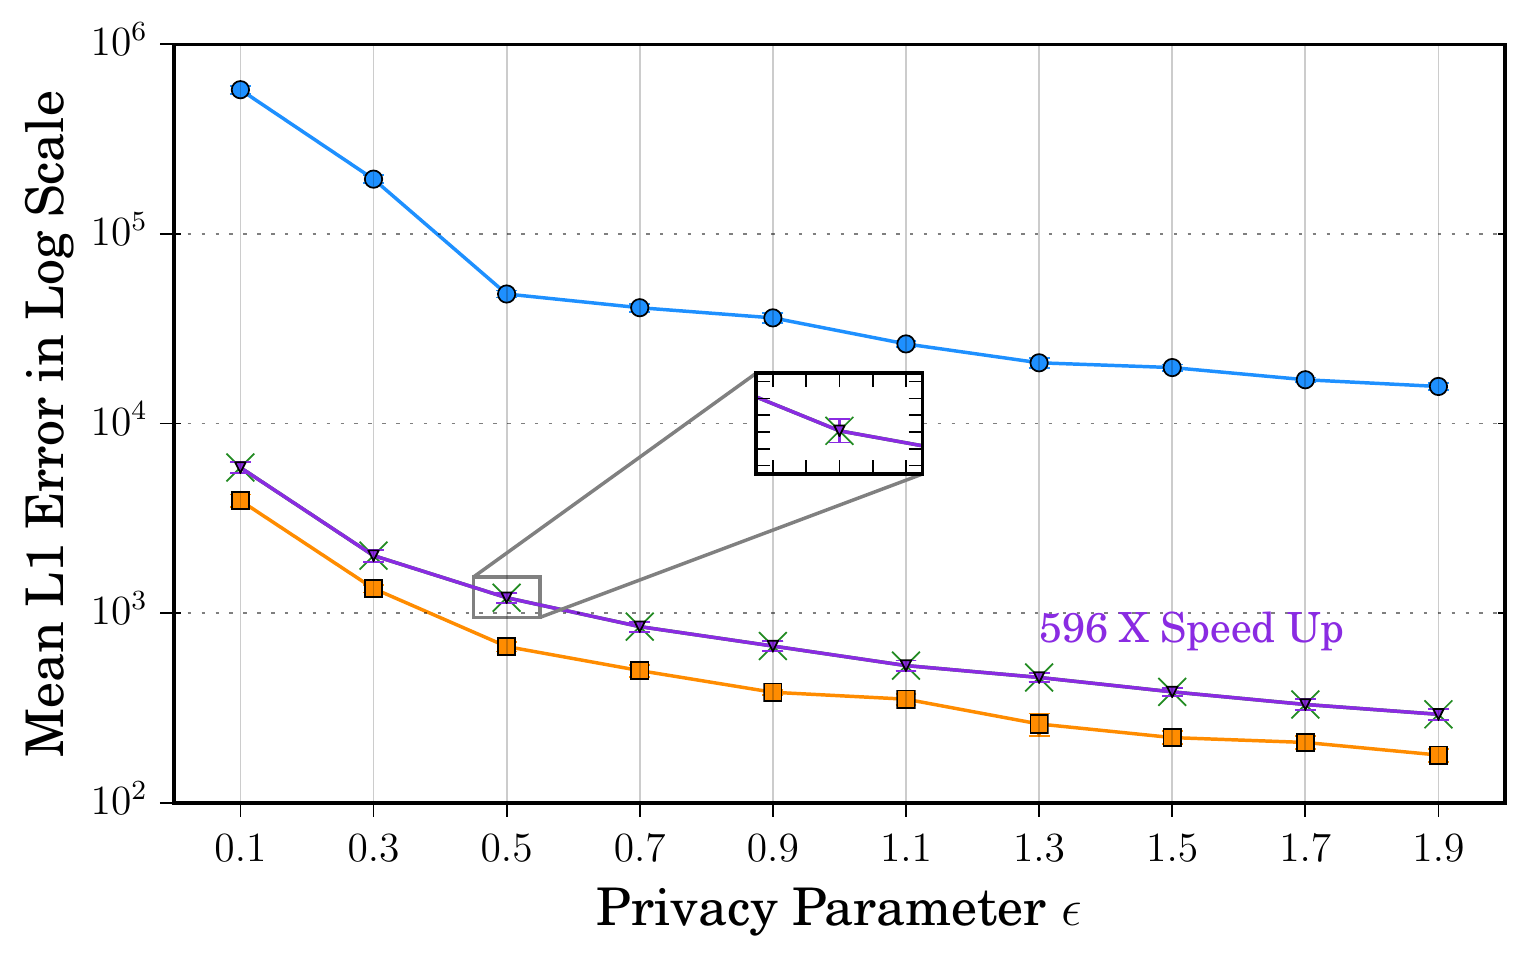}
        \caption{Program 3}
        \label{fig:P3}\end{subfigure}%%
    \begin{subfigure}[b]{0.25\linewidth}
    \centering    \includegraphics[width=1\linewidth]{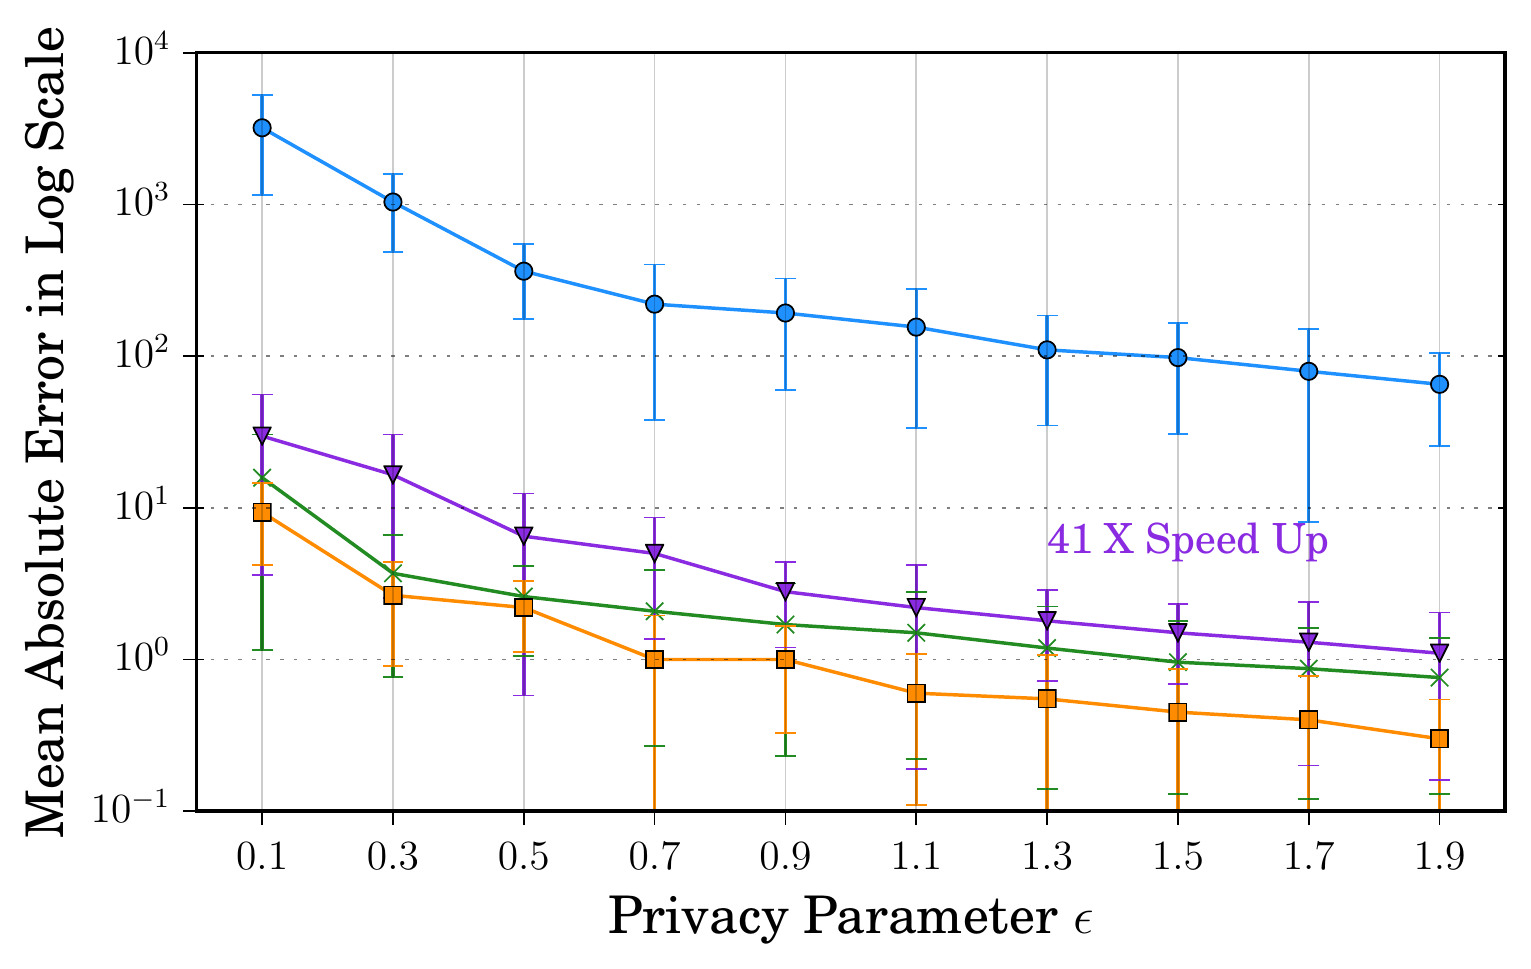}
        \caption{Program 5}
        \label{fig:P5}\end{subfigure}%%
      \begin{subfigure}[b]{0.25\linewidth}
    \centering    \includegraphics[width=1\linewidth]{7_final.pdf}
        \caption{Program 7}
        \label{fig:P7}
    \end{subfigure}
   \caption{Accuracy Analysis of Crypt$\epsilon$ Programs}
   \label{accuracy}
\end{figure*}
